# Supplementary material for: Strong anomalous diffusion for free-ranging birds
Source: arXiv:2411.04684 source file (2025-08-12)
Supplement: Supplementary file 1 [file Supplementary_Information_revision.pdf]

# Supplementary Information for Strong anomalous diffusion for free-ranging birds

Ohad Vilks<sup>a,b,\*</sup>, Motti Charter<sup>c</sup>, Sivan Toledo<sup>d</sup>, Eli Barkai<sup>e</sup>, Ran Nathan<sup>b</sup>

*a Racah Institute of Physics, The Hebrew University of Jerusalem, Jerusalem, Israel*

*b Movement Ecology Lab, Department of Ecology, Evolution and Behavior,*

*Alexander Silberman Institute of Life Sciences, Faculty of Science,*

*The Hebrew University of Jerusalem, Jerusalem, Israel.*

*c The Shamir Research Institute and School of Environmental Sciences,*

*University of Haifa, 199 Aba Hushi Boulevard, Mount Carmel, Haifa, Israel.*

*d Blavatnik School of Computer Science, Tel-Aviv University, Israel.*

*e Department of Physics, Institute of Nanotechnology and Advanced Materials,*

*Bar-Ilan University, Ramat-Gan 52900, Israel. and*

*\*To whom correspondence should be addressed: [ohad.vilk@mail.huji.ac.il](mailto:ohad.vilk@mail.huji.ac.il)*

In this supplementary information we provide Figs. S1-S5 to support the discussion in the main text. In what follows, the notations and abbreviations are the same as in the main text and the equations and figures refer to those therein.

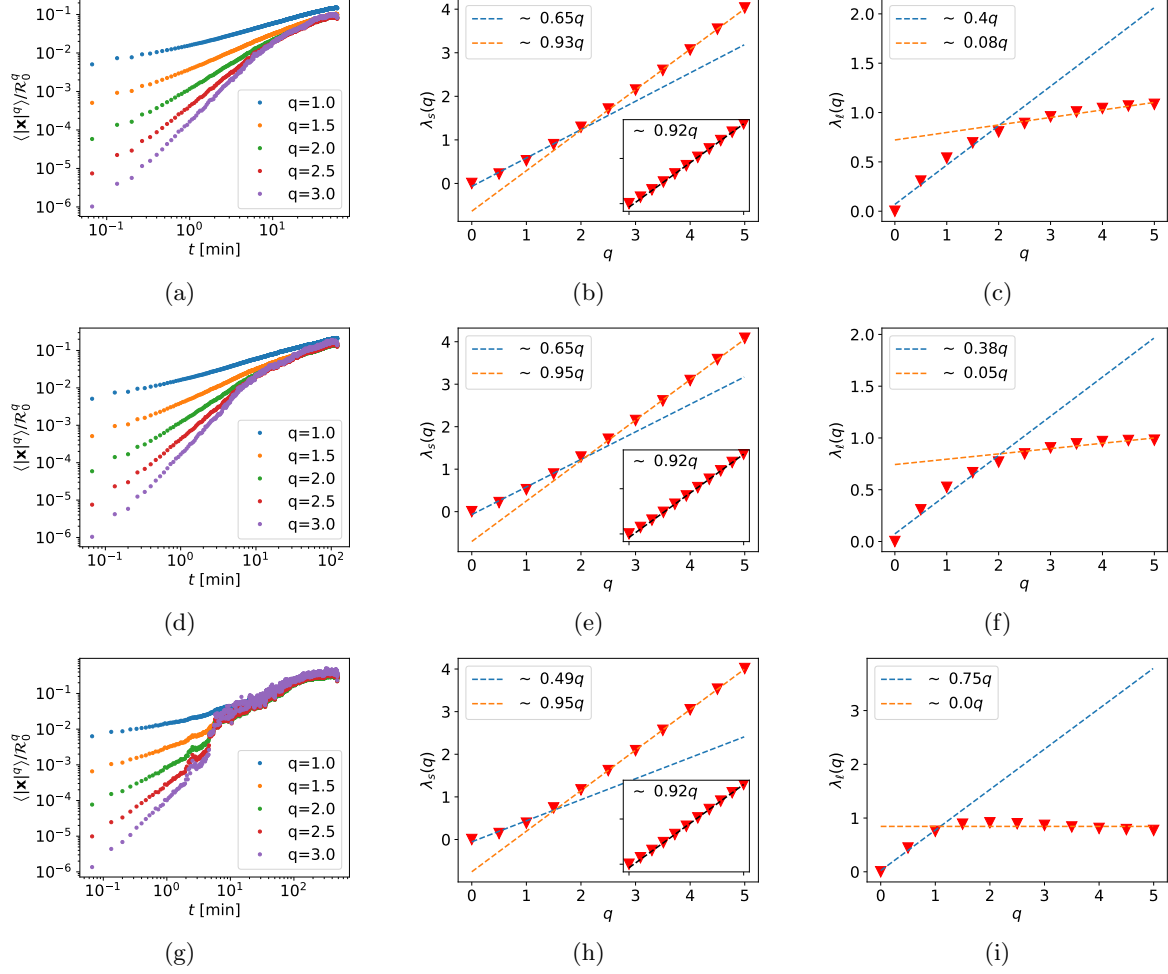

FIG. S1. Results for the adult Barn Owls based on tracks with different durations: (a-c) 1-hour, (d-f) 2-hour and (g-i) 8-hour. (a,d,g) Log-log plot of the average absolute displacement moments  $\langle |x(t) - x(0)|^q \rangle$ . Data points for moment orders  $q=1$  (blue),  $q=2$  (orange), and  $q=3$  (green) are shown. Circles represent empirical moments, while dashed lines indicate fits at short and long times. (b,e,h)  $\lambda_s(q)$  as a function of  $q$ . The red triangles represent the empirical values over short time intervals and the dashed blue and orange lines represent the bi-linear fit slopes for low and high moments, respectively. Inset:  $\lambda(q)$  for segmented commuting flights. (c,f,i)  $\lambda_\ell(q)$  as a function of  $q$  for long time intervals ( $> 5$  minutes, red triangles). The dashed blue and orange lines represent the bi-linear fit slopes for low and high moments, respectively.

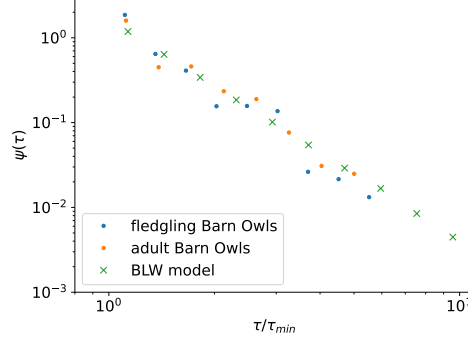

FIG. S2. Probability density function of jump times for adult and fledgling Barn Owls based on the segmentation detailed in the main text. The resulting distribution for both datasets are fitted to a power law and we find  $\alpha \simeq 1.6$ . The results are compared to BLW simulations ( $x$  marks) with  $\alpha = 1.6$ .

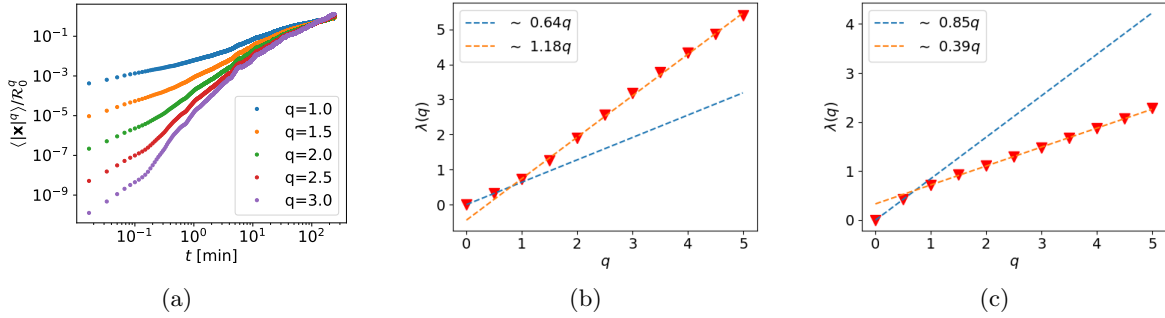

FIG. S3. Results for the multi-mode simulations for the fledgling's parameterization. (a) Log-log plot of the average absolute displacement moments  $\langle |\mathbf{x}|^q \rangle / \mathcal{R}_0^q$  with  $\mathcal{R}_0 = 2.5$  km representing the average maximum displacement of Barn Owls in a single night. Data points for moment orders  $q = 1, 1.5, 2, 2.5, 3$  are shown, displaying two distinct scaling regimes for each moment  $q$ , with a transition at  $\sim 5$  minutes. (b)  $\lambda_s(q)$  as a function of  $q$ . The red triangles represent the values over short time intervals of the simulations. The dashed blue and orange lines represent the bi-linear fit slopes for low and high moments, respectively, where the slopes are denoted in the legends. (c)  $\lambda_l(q)$  as a function of  $q$  for long time intervals ( $> 5$  minutes, red triangles). The dashed blue and orange lines represent the bi-linear fit slopes for low and high moments, respectively.

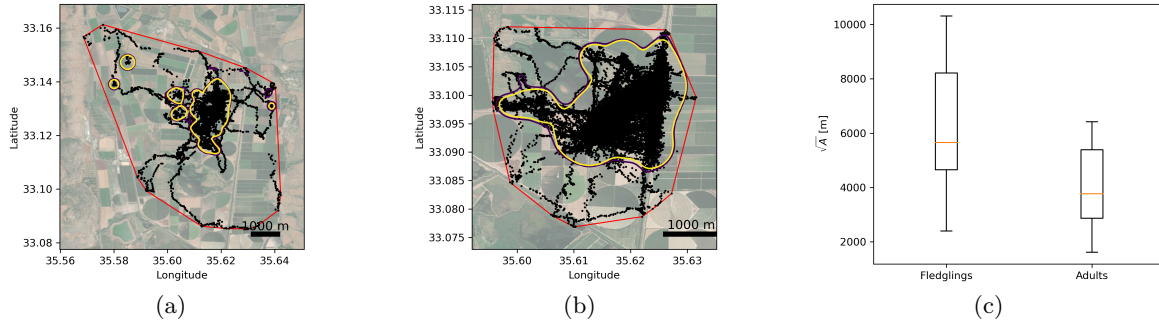

FIG. S4. Area estimation: comparison between fledgling and adult Barn Owls. Panel (a) shows the home range of a fledgling Barn Owl, tagged as 4722, with its movements overlaying a satellite map. Panel (b) presents the home range for an adult Barn Owl, tagged as 4915. In both panels, the black dots represent the movement track, the red line is an Minimum Convex Polygon (MCP) estimation of the home range, and the yellow and purple lines indicate the 68th and 95th percentiles of the home range estimated using Kernel Density Estimation (KDE). Panel (c) compares the squared root of the home range areas – as inferred from the MCP – between fledglings and adults.
